# Supplementary material for: Strong-field photoionization by circularly polarized light
Source: arXiv:2306.12999 source file (2023-06-22)
Supplement: Supplementary file 1 [file supplemental_material.pdf]

# – Supplemental Material –
# Strong field photoionization by circularly polarized light

Jonathan Dubois,[1,2] Camille Lévêque,[1] Jérémie Caillat,[1] Richard Taïeb,[1] Ulf Saalmann,[2] and Jan-Michael Rost[2]

[1]*Sorbonne Université, CNRS, Laboratoire de Chimie Physique – Matière et Rayonnement, LCPMR, 75005 Paris, France*
[2]*Max Planck Institute for the Physics of Complex Systems, Nöthnitzer Straße 38, 01187 Dresden, Germany*

## I. ION-ELECTRON POTENTIALS

Throughout the article, we use the ion-electron potential

$$V(\mathbf{r}) = -\frac{1}{\sqrt{|\mathbf{r}|^2 + a^2}}, \qquad a = 0.26, \tag{SM1a}$$

for He [1] and

$$V(\mathbf{r}) = -\frac{1 + 9\exp(-|\mathbf{r}|^2)}{\sqrt{|\mathbf{r}|^2 + a^2}}, \qquad a = 1.70, \tag{SM1b}$$

for Ne [2]. Numerically, the initial state wavefunctions $\psi_0$ and $I_p$ for each model atom were obtained using imaginary-time propagation [3].

## II. ELECTRON IONIZATION POTENTIAL IN THE RF

The initial energy in the LF in absence of laser field is given by the eigenvalue problem

$$\mathrm{H}_0\psi_0 = -I_p\psi_0, \tag{SM2}$$

where

$$\mathrm{H}_0 = \frac{\mathbf{p}^2}{2} + V(\mathbf{r}). \tag{SM3}$$

Due to the time-dependence of the unitary transformation from the LF to the RF, the Hamiltonian in the RF is given by

$$\widetilde{\mathrm{H}}_0 = \mathrm{H}_0 - \omega\,\mathrm{L}_z. \tag{SM4}$$

The initial state is such that $\mathrm{L}_z\psi_0{=}m\psi_0$ where $m$ is the magnetic quantum number. As a consequence, the eigenvalue problem in the RF becomes

$$\widetilde{\mathrm{H}}_0\psi_0 = -(I_p + m\omega)\psi_0. \tag{SM5}$$

The ionization potential of the electron in the RF is therefore

$$\widetilde{I}_p = I_p + m\omega, \tag{SM6}$$

and depends explicitly on the magnetic quantum number and the frequency of the circularly polarized laser field.

## III. KINETIC AND POTENTIAL ENERGIES IN THE RF

The Hamiltonian in the RF is given by

$$\widetilde{\mathrm{H}}(t) = \frac{\mathbf{p}^2}{2} + V(\mathbf{r}) - \omega\mathrm{L}_z + \mathbf{r}\cdot\widetilde{\mathbf{F}}(t), \tag{SM7}$$

and reads also as

$$\widetilde{\mathrm{H}}(t) = \frac{1}{2}\Big(\mathbf{p} - \omega \mathbf{e}_z \times \mathbf{r}\Big)^2 + V(\mathbf{r}) - \frac{\omega^2}{2}\big(\mathbf{e}_z \times \mathbf{r}\big)^2 + \mathbf{r}\cdot\widetilde{\mathbf{F}}(t), \tag{SM8}$$

and therefore the kinetic term is

$$\widetilde{K} = \frac{1}{2}\Big(\mathbf{p} - \omega \mathbf{e}_z \times \mathbf{r}\Big)^2, \tag{SM9}$$

and the effective potential is

$$\widetilde{V}_{\text{eff}}(t) = V(\mathbf{r}) - \frac{\omega^2}{2}\big(\mathbf{e}_z \times \mathbf{r}\big)^2 + \mathbf{r}\cdot\widetilde{\mathbf{F}}(t). \tag{SM10}$$

## IV. GREEN FUNCTION IN THE LABORATORY FRAME AND IN THE ROTATING FRAME

### A. Laboratory frame

The Green function for the linear operator on the left- hand side of (8a) can be expressed in terms of the classical action $\mathcal{S}$, which is exact since the operator $\mathrm{H}(t)$ is linear in position for $V{=}0$ [4, 5],

$$G(\mathbf{r},t;\mathbf{r}',t') = -\mathrm{i}\Theta(t-t')\left(\det\left(\frac{1}{2\mathrm{i}\pi}\frac{\partial^2\mathcal{S}}{\partial\mathbf{r}\partial\mathbf{r}'}\right)\right)^{1/2}\exp\Big(\mathrm{i}\mathcal{S}(\mathbf{r},t;\mathbf{r}',t')\Big), \tag{SM11}$$

with $\Theta$ the Heaviside step function and $\mathcal{S}$ the classical action of the electron explicitly given by

$$\mathcal{S}(\mathbf{r},t;\mathbf{r}',t') = \frac{\Big(\mathbf{r}-\mathbf{r}'-\int_{t'}^{t}\mathbf{A}(\tau)\,\mathrm{d}\tau\Big)^2}{2(t-t')} + \mathbf{r}\cdot\mathbf{A}(t) - \mathbf{r}'\cdot\mathbf{A}(t') - \frac{1}{2}\int_{t'}^{t}\mathbf{A}(\tau)^2\,\mathrm{d}\tau. \tag{SM12}$$

### B. Rotating frame

#### 1. General laser pulse

In the RF, the Green function and the classical action become

$$\widetilde{G}(\mathbf{r},t;\mathbf{r}',t') = G(R_\omega^{-1}(t)\mathbf{r},t;R_\omega^{-1}(t')\mathbf{r}',t'), \tag{SM13}$$
$$\widetilde{\mathcal{S}}(\mathbf{r},t;\mathbf{r}',t') = \mathcal{S}(R_\omega^{-1}(t)\mathbf{r},t;R_\omega^{-1}(t')\mathbf{r}',t'), \tag{SM14}$$

with

$$R_\omega(t) = \begin{pmatrix} \cos(\omega t) & \sin(\omega t) & 0 \\ -\sin(\omega t) & \cos(\omega t) & 0 \\ 0 & 0 & 1 \end{pmatrix}, \tag{SM15}$$

and therefore (using $R_\omega(t)R_\omega^{-1}(t'){=}R_\omega(t{-}t')$)

$$\widetilde{\mathcal{S}}(\mathbf{r},t;\mathbf{r}',t') = \frac{\Big(\mathbf{r}-R_\omega(t-t')\mathbf{r}'-R_\omega(t)\int_{t'}^{t}\mathbf{A}(\tau)\,\mathrm{d}\tau\Big)^2}{2(t-t')} + \mathbf{r}\cdot\widetilde{\mathbf{A}}(t) - \mathbf{r}'\cdot\widetilde{\mathbf{A}}(t') - \frac{1}{2}\int_{t'}^{t}\widetilde{\mathbf{A}}(\tau)^2\,\mathrm{d}\tau, \tag{SM16}$$

where $\widetilde{\mathbf{A}}(t){=}R_\omega(t)\mathbf{A}(t)$.

### 2. *Constant envelope*

For circularly polarized pulses with constant envelope, the vector potential and electric field of the laser are

$$\mathbf{A}(t) = \frac{F}{\omega}\Big(\mathbf{e}_x \cos(\omega t) + \mathbf{e}_y \sin(\omega t)\Big), \tag{SM17}$$

$$\mathbf{F}(t) = F\Big(\mathbf{e}_x \sin(\omega t) - \mathbf{e}_y \cos(\omega t)\Big), \tag{SM18}$$

and therefore they are constant in the RF

$$\widetilde{\mathbf{A}} = R_\omega(t)\mathbf{A}(t) = \frac{F}{\omega}\mathbf{e}_x, \tag{SM19}$$

$$\widetilde{\mathbf{F}} = R_\omega(t)\mathbf{F}(t) = -F\mathbf{e}_y. \tag{SM20}$$

In addition,

$$\int_{t'}^{t} \mathbf{A}(\tau)\mathrm{d}\tau = \frac{1}{\omega^2}\Big(\mathbf{F}(t) - \mathbf{F}(t')\Big). \tag{SM21}$$

Therefore,

$$R_\omega(t)\int_{t'}^{t} \mathbf{A}(\tau)\mathrm{d}\tau = \frac{1}{\omega^2}\Big(\mathbb{I} - R_\omega(t-t')\Big)\widetilde{\mathbf{F}}, \tag{SM22}$$

where $\mathbb{I}$ is the identity. Finally, the classical action in the RF for a circularly polarized pulse with a constant envelope is given by

$$\widetilde{\mathcal{S}}(\mathbf{r},t;\mathbf{r}',t') = \frac{\left(\left(\mathbf{r} - \frac{\widetilde{\mathbf{F}}}{\omega^2}\right) - R_\omega(t-t')\left(\mathbf{r}' - \frac{\widetilde{\mathbf{F}}}{\omega^2}\right)\right)^2}{2(t-t')} + \Big(\mathbf{r} - \mathbf{r}'\Big)\cdot\widetilde{\mathbf{A}} - \frac{\widetilde{\mathbf{A}}^2}{2}(t-t'). \tag{SM23}$$

The classical action, and therefore the Green function, are invariant under time translation.

---


[1] F. Mauger, A. D. Bandrauk, A. Kamor, T. Uzer, and C. Chandre, Journal of Physics B: Atomic, Molecular and Optical Physics **47**, 041001 (2014).

[2] I. Barth and M. Lein, J. Phys. B: At. Mol. Opt. Phys. **47**, 204016 (2014).

[3] A. D. Bandrauk, E. Dehghanian, and H. Lu, Chemical Physics Letters **419**, 346 (2006).

[4] R. G. Littlejohn, Journal of Statistical Physics **68**, 7 (1992).

[5] R. G. Littlejohn, Physics Reports **138**, 193 (1986).
